# Supplementary material for: Microscopic mechanism for the shear-thickening of non-Brownian suspensions
Source: arXiv:1308.1002 source file (2013-08-05)
Supplement: Supplementary file 1 [file Isa_SI.pdf]

# Microscopic mechanism for the shear-thickening of non-Brownian suspensions SUPPLEMENTAL MATERIAL

Nicolas Fernandez,[1] Roman Mani,[2] David Rinaldi,[3] Dirk Kadau,[2] Martin Mosquet,[3] Hélène Lombois-Burger,[3] Juliette Cayer-Barrioz,[4] Hans J. Herrmann,[2] Nicholas D. Spencer,[1] and Lucio Isa[1,*]

[1]*Laboratory for Surface Science and Technology, Department of Materials, ETH Zurich, Switzerland*
[2]*Computational Physics for Engineering Materials, Department of Civil, Environmental and Geomatic Engineering, ETH Zurich, Switzerland*
[3]*Lafarge LCR, Saint Quentin-Fallavier, France*
[4]*Laboratoire de Tribologie et Dynamique des Systèmes - UMR 5513 CNRS, École Centrale de Lyon, France*

## NUMERICAL SIMULATIONS

### Friction law calculation

In order to simulate our dense paste we need to model the behavior of the particles and the fluid. We assume that the fluid layers between particles are very thin compared to the particle radius and of the same order of magnitude as the amplitude of their surface roughness. This assumption allows us to avoid solving explicit equations for the suspending fluid, which are extremely computationally expensive even for a single contact. It also permits the use of a local friction law that takes into account the lubrication effect of the suspending fluid in the form of the well-known Stribeck curve. The system can then be easily simulated with contact dynamics.

A typical Stribeck curve shows two main lubrication regimes separated by a "mixed" zone: a boundary lubrication (BL) regime where the asperities on the two sliding surfaces are in contact and a hydrodynamically lubricated (HD) regime where the shear of the fluid film is responsible for energy dissipation. Implementing boundary lubrication is straightforward in simulations because the friction coefficient in this regime is usually independent of the speed and the load. The novelty in our simulations is the implementation of the hydrodynamic regime in the particle-particle contact friction law.

As already reported in the main body of the article, the hydrodynamic interactions between two similar neighboring spheres in the HD regime are described by standard low-Reynolds-number fluid mechanics with a lubrication hypothesis (i.e. inter-surface distance small compared to the radius of the particle). The drag force on one particle due to the other is given in the canonical reference frame of the contact by (for overall formula [1] and for detailed calculations: diagonal terms [2] and the non-diagonal term [3]) :

$$\mathbf{F}_{1\to 2}^{HD} = \frac{\pi}{10}\eta_f R_p \begin{bmatrix} -15h^{-1} & 12h^{-\frac{1}{2}} \\ 0 & -10ln(h^{-1}) \end{bmatrix} \begin{bmatrix} v_N \\ v_T \end{bmatrix} \quad (1)$$

where $h$ is the surface-to-surface distance normalized by $R_p$, $\eta_f$ is the fluid viscosity and $v_N$ and $v_T$ are the normal and tangential components of the local relative speed respectively. By definition of the reference frame: $v_T \geq 0$. Please note that spinning around the normal direction is neglected because other components of the drag dominate for small $h$, i.e. the normal spinning drag does not diverge when $h \longrightarrow 0$ [4].

Additionally, the typical Reynolds numbers of the particle $Re_p = \frac{\rho_p R_p^2 \dot{\gamma}}{\eta_f}$ (with $\rho_p$ being the density of the particle) are small for the range of shear rates that we investigate experimentally. Inertia effects are thus negligible and only the steady-state lubrication is relevant. Moreover, the particles cannot interpenetrate each other and the existence of a long-lived contact itself implies that $v_N = 0$, given that for $v_N > 0$ the particles leave each other. This hypothesis is justified by prior simulation studies, in which the contact duration between particles in dense granular media was long compared to $\dot{\gamma}^{-1}$ [5]. As an additional consequence of this hypothesis, the shear thickening that we observe cannot be due to some hydroclusters that are arising from attractive viscous forces in opening contacts.

With these hypotheses, Newton's second law on one of the spheres, projected on the normal and tangential axis of the contact, becomes:

$$\frac{6\pi\eta_f R_p}{5\sqrt{h}} v_T + F_N^{ext} = 0 \quad (2)$$

$$-\pi\eta_f R_p ln(h^{-1}) v_T + F_T^{ext} = 0 \quad (3)$$

with $F_N^{ext}$ and $F_T^{ext}$ being the sums of external forces applied on the sphere by means of other contacts projected on the normal and tangential axes.

At this stage, following standard hydrodynamic lubrication analysis [6], the minimum thickness of the fluid layer between the contacting particles is given by equation (2):

$$h = (\frac{6\pi}{5}s)^2 \quad (4)$$

with $s$, the Sommerfeld number as defined in the paper. The ratio between the tangential viscous drag and the

normal load gives the coefficient of friction $\mu$ reported in the main body of the paper:

$$\mu = \frac{\|F_T^{ext}\|}{\|F_N^{ext}\|} = 2\pi s ln(\frac{5}{6\pi s}) \quad (5)$$

As already explained in the main article, this formula is valid only for small $s$ because the lubrication hypothesis is valid only for $h \propto s^2 << 1$. We fixed the validity limit of equation (5) at $s_{lim} = 10^{-1}$ and $\mu(s) = \mu(s_{lim})$ for $s > s_{lim}$. In any case we have demonstrated in the numerical simulations that there are less than 0.5% of the contacts with $s > 10^{-1}$ in the considered range of shear stresses and that the resulting forces are weak.

Finally, as an additional consequence of the long-lived contact hypothesis, the normal restitution coefficient, $e_N$, is zero for both lubrication regimes. It can be seen physically as the result of the intense damping of any normal speed when two particles are near each other, as seen in Eq.1. Moreover, the normal restitution coefficient is known to have a minor impact on the behavior of dense granular media [7].

## Variation of the parameters

In the simulations, the stress $\tau$, the shear rate $\dot{\gamma}$ and the apparent viscosity $\eta$ can be tuned by varying the dimensionless number

$$\lambda = \frac{\sqrt{\tau\rho}R}{\eta_f} \quad (6)$$

The time scale of the problem is set by $[T] = \sqrt{\rho/\tau}R$ and thus, we can introduce the dimensionless shear rate $\dot{\gamma}$, velocity $\tilde{v}$ and load $\tilde{N}$ via

$$\dot{\gamma} = \tilde{\dot{\gamma}}\frac{\sqrt{\tau/\rho}}{R} = \tilde{\dot{\gamma}}\lambda\frac{\eta_f}{\rho R^2}$$
$$v = \tilde{v}\sqrt{\frac{\tau}{\rho}} \quad (7)$$
$$N = \tilde{N}\tau R^2$$

The Sommerfeld number can be expressed as

$$s = \eta_f\frac{vr}{N} = \eta_f\frac{\tilde{v}r}{\tilde{N}\sqrt{\rho\tau}R^2} = \frac{\tilde{v}r}{\tilde{N}R\lambda} = \tilde{r}\frac{\tilde{v}}{\tilde{N}}\lambda^{-1} \quad (8)$$

where $r = \tilde{r}R$ is the normalized particle radius. For unequal spheres, we assume that we can replace $r$ by the average radius $2r_c^{-1} = r_1^{-1} + r_2^{-1}$ such that

$$s = \tilde{r}_c\frac{\tilde{v}}{\tilde{N}}\lambda^{-1} \quad (9)$$

Here, we readily see that for fixed $\phi, \mu_0, s_c$ the only control parameter is $\lambda$. In our simulations, we varied $\lambda$ to obtain $\tilde{\dot{\gamma}}$ as the simulation output. From Eq. (6) the stress $\tau$ is obtained via $\tau = \lambda^2\eta_f^2/(\rho R^2)$ such that the apparent viscosity is given by

$$\eta = \frac{\tau}{\dot{\gamma}} = \frac{\lambda}{\tilde{\dot{\gamma}}}\eta_f \quad (10)$$

## Role of the lubricating fluid

As outlined in the main article, the observation of a transition from a Newtonian to a shear thickening regime relies on the presence of a lubricating fluid. Now we show that, also in the numerical model, it is essential to include a lubricating contact law in order to observe this kind of transition. Fig. 1 shows data from the main article superimposed to simulations where the lubrication is disregarded, i.e. $\mu = const$, or in other words, all contacts are always in the boundary lubrication regime. Here, we see that the curve $\mu = 0.2 = const$ exhibits pure Bagnoldian scaling for any shear rate $\dot{\gamma}$ and coincides at large $\dot{\gamma}$ with the data where lubrication is taken into account (curve $\mu_0 = 0.2$). For $\mu = const$, there is no transition to a Newtonian regime. Furthermore, the vertical solid line indicates that the system is jammed at any applied stress for $\mu = 0.4 = const$ as opposed to lubricated contacts where flow is possible at sufficiently low $\dot{\gamma}$ (see $\mu_0 = 0.4$). Note that as we consider infinitely hard particles in our simulations, the jamming point does not depend on the applied stress as opposed to soft sphere simulations as in Ref. [8].

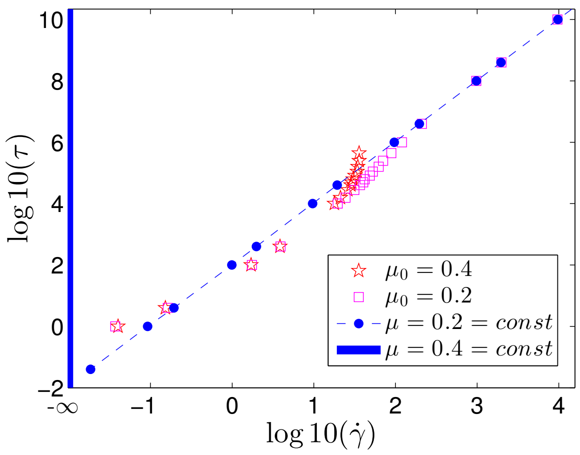


FIG. 1. Shear stress $\tau$ as a function of $\dot{\gamma}$ for two different friction coefficients. Stars and squares correspond to data where the lubrication is taken into account in the numerical model, whereas filled circles correspond to a constant $\mu$, i.e. lubrication is disregarded. The solid line schematically shows the jammed state, where no flow is possible at any applied stress when lubrication is disregarded.

### Effect of confining walls

In order to investigate the influence of the confining walls, we also modified the boundary conditions in the vertical $z$-direction by removing the walls and using Lees-Edwards [9] boundary conditions instead. Shear in $x$-direction is induced by considering moving (in $x$-direction) mirror images of the simulation box. Shortly speaking, particles at the bottom of the simulation box interact with particles at the top of the box, which have an $x$ coordinate displaced by an amount $\delta_x = tv_{shear}$ where $v_{shear}$ is the shearing velocity and $t$ is time. When particles cross the boundaries in $z$-direction, the $x$-velocities are corrected by an amount $\delta_v = v_{shear}$. As in the main article, we simulate stress-controlled shearing at mean stress $\tau_0$ where the shearing velocity $v_{shear}$ is measured. In order to keep a constant mean stress, $v_{shear}$ is adjusted via the equation of motion $\dot{v}_{shear} = (\tau_0 - \tau)$ [10] where $\tau = -1/V \sum_i F_x^i r_z^i$ is the actual shear stress of the sample. The sum runs over all contacts $i$ having contact force $F_i$ and distance vector $r_i$ connecting the two centers of the spheres. The effective viscosity of the suspension is given by $\eta = \tau_0/\dot{\gamma}$ where $\dot{\gamma} = v_{shear}/L_z$ and $L_z$ is the system size in $z$-direction.

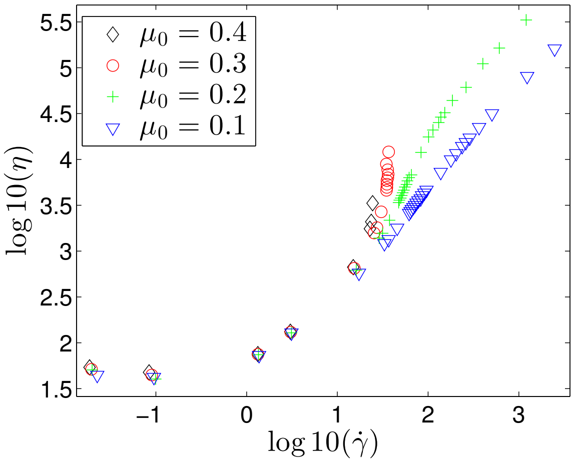


FIG. 2. Effective viscosity as a function of the shear rate for different $\mu_0$ at $\phi = 0.595$ for a system with periodic boundary conditions in all three directions.

Fig. 2 shows $\eta$ as a function of $\dot{\gamma}$ for different boundary lubrication friction coefficients $\mu_0$ and volume fraction $\phi = 0.595$. As in the main article, we observe two transitions, from Newtonian to Bagnold as $\dot{\gamma}$ is increased and from continuous to discontinuous shear thickening as $\mu_0$ is increased. These calculations suggest indeed that friction law is responsible for both the different observed flow regimes and the transitions between them. In particular the DST transition is not due to the presence of confining walls. The critical volume fraction and $\mu_0$ at which the system experiences DST are slightly larger compared to the values in the main article, but no qualitative differences are found. This is due to the fact that the presence of hard walls has the effect of reducing the accessible volume to the particles in the system [8].

## POLYMER ADDITION AND RHEOLOGY

In shear rheology, any addition of small quantities of adsorbing polymers decreases the viscosity, both in the low-(deflocculation) and high-shear-rate (ST) regimes. Above a certain mass of polymer per unit mass of quartz, further addition of polymer no longer changes the suspension viscosity. This saturation takes place at polymer concentrations in the solution below 2 $\%_{mass}$, thus far below levels that could change the viscosity of the suspending fluid. All the rheology experiments were thus carried out with excess polymer relative to the saturation mass ratio.

The working polymer mass ratios were $r(A) = 3.1$ $mg/g_{SiO_2}$, $r(B) = 3.1$ $mg/g_{SiO_2}$, $r(C) = 1.5$ $mg/g_{SiO_2}$ and $r(D) = 4.0$ $mg/g_{SiO_2}$. These working concentrations have not been precisely optimized, nevertheless the small value of $r(C)$ can be explained by polymer C shorter side chains that create a thinner brush layer and thus a lower adsorbed mass per unit surface [11]. In addition to 20 $mmol/L$ of $K_2SO_4$, an excess of $Ca(OH)_2$ (6 $mg/g_{SiO_2}$) was added to maintain saturation of the buffer solution even after the reaction of $OH^-$ with the surface of the quartz grains and the adsorption of calcium ions. In similar conditions, the $\zeta$-potential of silica surfaces have been reported to be around 6mV [12]. A drop of Surfynol MD-20 (antifoaming Gemini surfactant, from Air Products, USA) was also added to prevent air trapping during the mixing.

Even if the adsorption of the polymers seemed immediate, the experiments were performed at least 10 min after the initial mixing. During this period the suspension can settle a bit, the suspension is then homogenize by mixing and by the pre-shear (increasing logarithmic stress ramp from 0.01 to 700 $Pa$ in 100 $s$ for the shear rheology, and 5 min of whirly mixing)

## FRICTION MEASUREMENTS

The friction between quartz grains cannot be directly and accurately measured due to their size and their complex shape. In order to establish the difference between the lubrication ability of the four tested polymers, the friction force was measured on a model tribosystem, a borosilicate glass sphere with a radius of 2 mm (from Sigma-Aldrich) and a polished quartz plane. The stone was polished using a set of decreasing SiC polishing papers and diamond pastes down to 1$\mu m$-grade (from

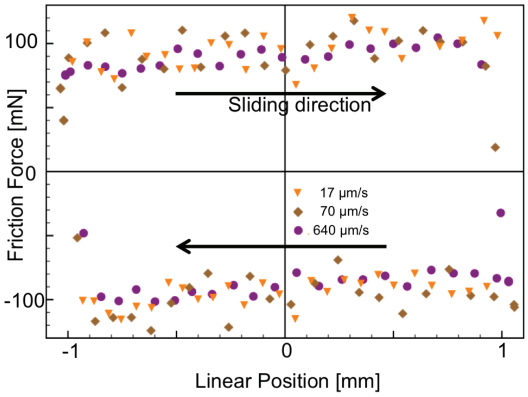


FIG. 3. Friction force for the 3 sliding speeds and a constant load of 100 mN on one cycle of amplitude 2mm for polymer C. Each value was recorded over a $8\mu m$ sliding distance (due to time resolution of the apparatus) but only 50 values per speed (equally spaced) are plotted

Struers, Denmark). Then the polished stone and the spheres were cleaned for 20 min using Piranha solution (7:3 concentrated $H_2SO_4$/30% $H_2O_2$). The sliding surfaces were immersed without contact between each other in the drop of the polymer alkali solution (100 $\mu L$, polymer concentration of 5 $\%_{mass}$) for 10 min before the beginning of the measurement. The polymers are adsorbed on both surfaces via calcium bridging under alkali conditions. In addition, in order to prevent acidification of the solution by $CO_2$ dissolution, the measurements were performed under a $N_2$ atmosphere at room pressure and temperature. Neither modification of pH nor $CaCO_3$ precipitation was observed during the experiments. The experiments were carried out at a sliding velocity of 640, 70 and 17 $\mu m/s$ under a constant load of 100 mN over a 2 mm long track under reciprocating conditions. Under these conditions, according to Hertz' theory [6], the average local pressure is around $0.1GPa$ and the expected contact radius is $16\mu m$, which remains small compared to the sliding distance.

Between two measurements, the sphere was renewed and the quartz surface was washed using a large volume of neutral pH buffer solution and then pure water (Milli-Q system from Millipore, 18.2 $M\Omega.cm$) in order to desorb and remove the polymer without modifying the quartz surfaces by aggressive chemical and thermal cleaning procedures. As stated in the paper and shown in Fig.3, the friction force does not depend on the sliding velocity and is stable with time. The average friction coefficient is then calculated over a distance of 1.2 mm.

* Corresponding author: lucio.isa@mat.ethz.ch

[1] P. Coussot and C. Ancey, *Rhéophysique des pâtes et des suspensions* (EDP Sciences, 1999).
[2] S. Kim and S. J. Karrila, Butterworth-Heinemann (1991).
[3] J. Howlett, Journal of Applied Physics **17**, 137 (1946).
[4] R. W. Snidle and J. F. Archard, Proceedings of the Institution of Mechanical Engineers **184**, 839 (1969).
[5] Y. Forterre and O. Pouliquen, Annual Review of Fluid Mechanics , 1 (2008).
[6] G. W. Stachowiak and A. W. Batchelor, *Engineering tribology* (Butterworth-Heinemann, 2005).
[7] F. Da Cruz, F. Chevoir, J. N. Roux, and I. Iordanoff, Tribology Series , 53 (2003).
[8] M. P. Ciamarra, R. Pastore, M. Nicodemi, and A. Coniglio, Physical Review E **84** (2011), 10.1103/PhysRevE.84.041308.
[9] M. P. Allen and D. J. Tildesley, *Computer Simulation of Liquids*, Oxford Science Publications (Oxford University Press, USA, 1989).
[10] M. Otsuki and H. Hayakawa, Physical Review E **83**, 051301 (2011).
[11] S. S. Perry, X. Yan, F. T. Limpoco, S. Lee, M. Müller, and N. D. Spencer, ACS Applied Materials & Interfaces **1**, 1224 (2009).
[12] C. Schroefl, M. Gruber, M. Lesti, and R. Sieber, Journal of Advanced Concrete Technology **7**, 5 (2009).
